# Supplementary material for: Relation-Aware Language-Graph Transformer for Question Answering
Source: arXiv:2212.00975 source file (2023-04-25)
Supplement: Supplementary file 1 [file obqa_leaderboard.tex]

\input{Tables/obqa_leaderboard.tex}
