# Supplementary material for: Relation-Aware Language-Graph Transformer for Question Answering
Source: arXiv:2212.00975 source file (2023-04-25)
Supplement: Supplementary file 2 [file qualitative_analysis.tex]

\paragraph{Qualitative analyses.}
\begin{figure}[t!]
\begin{center}
\includegraphics[width=1\columnwidth]{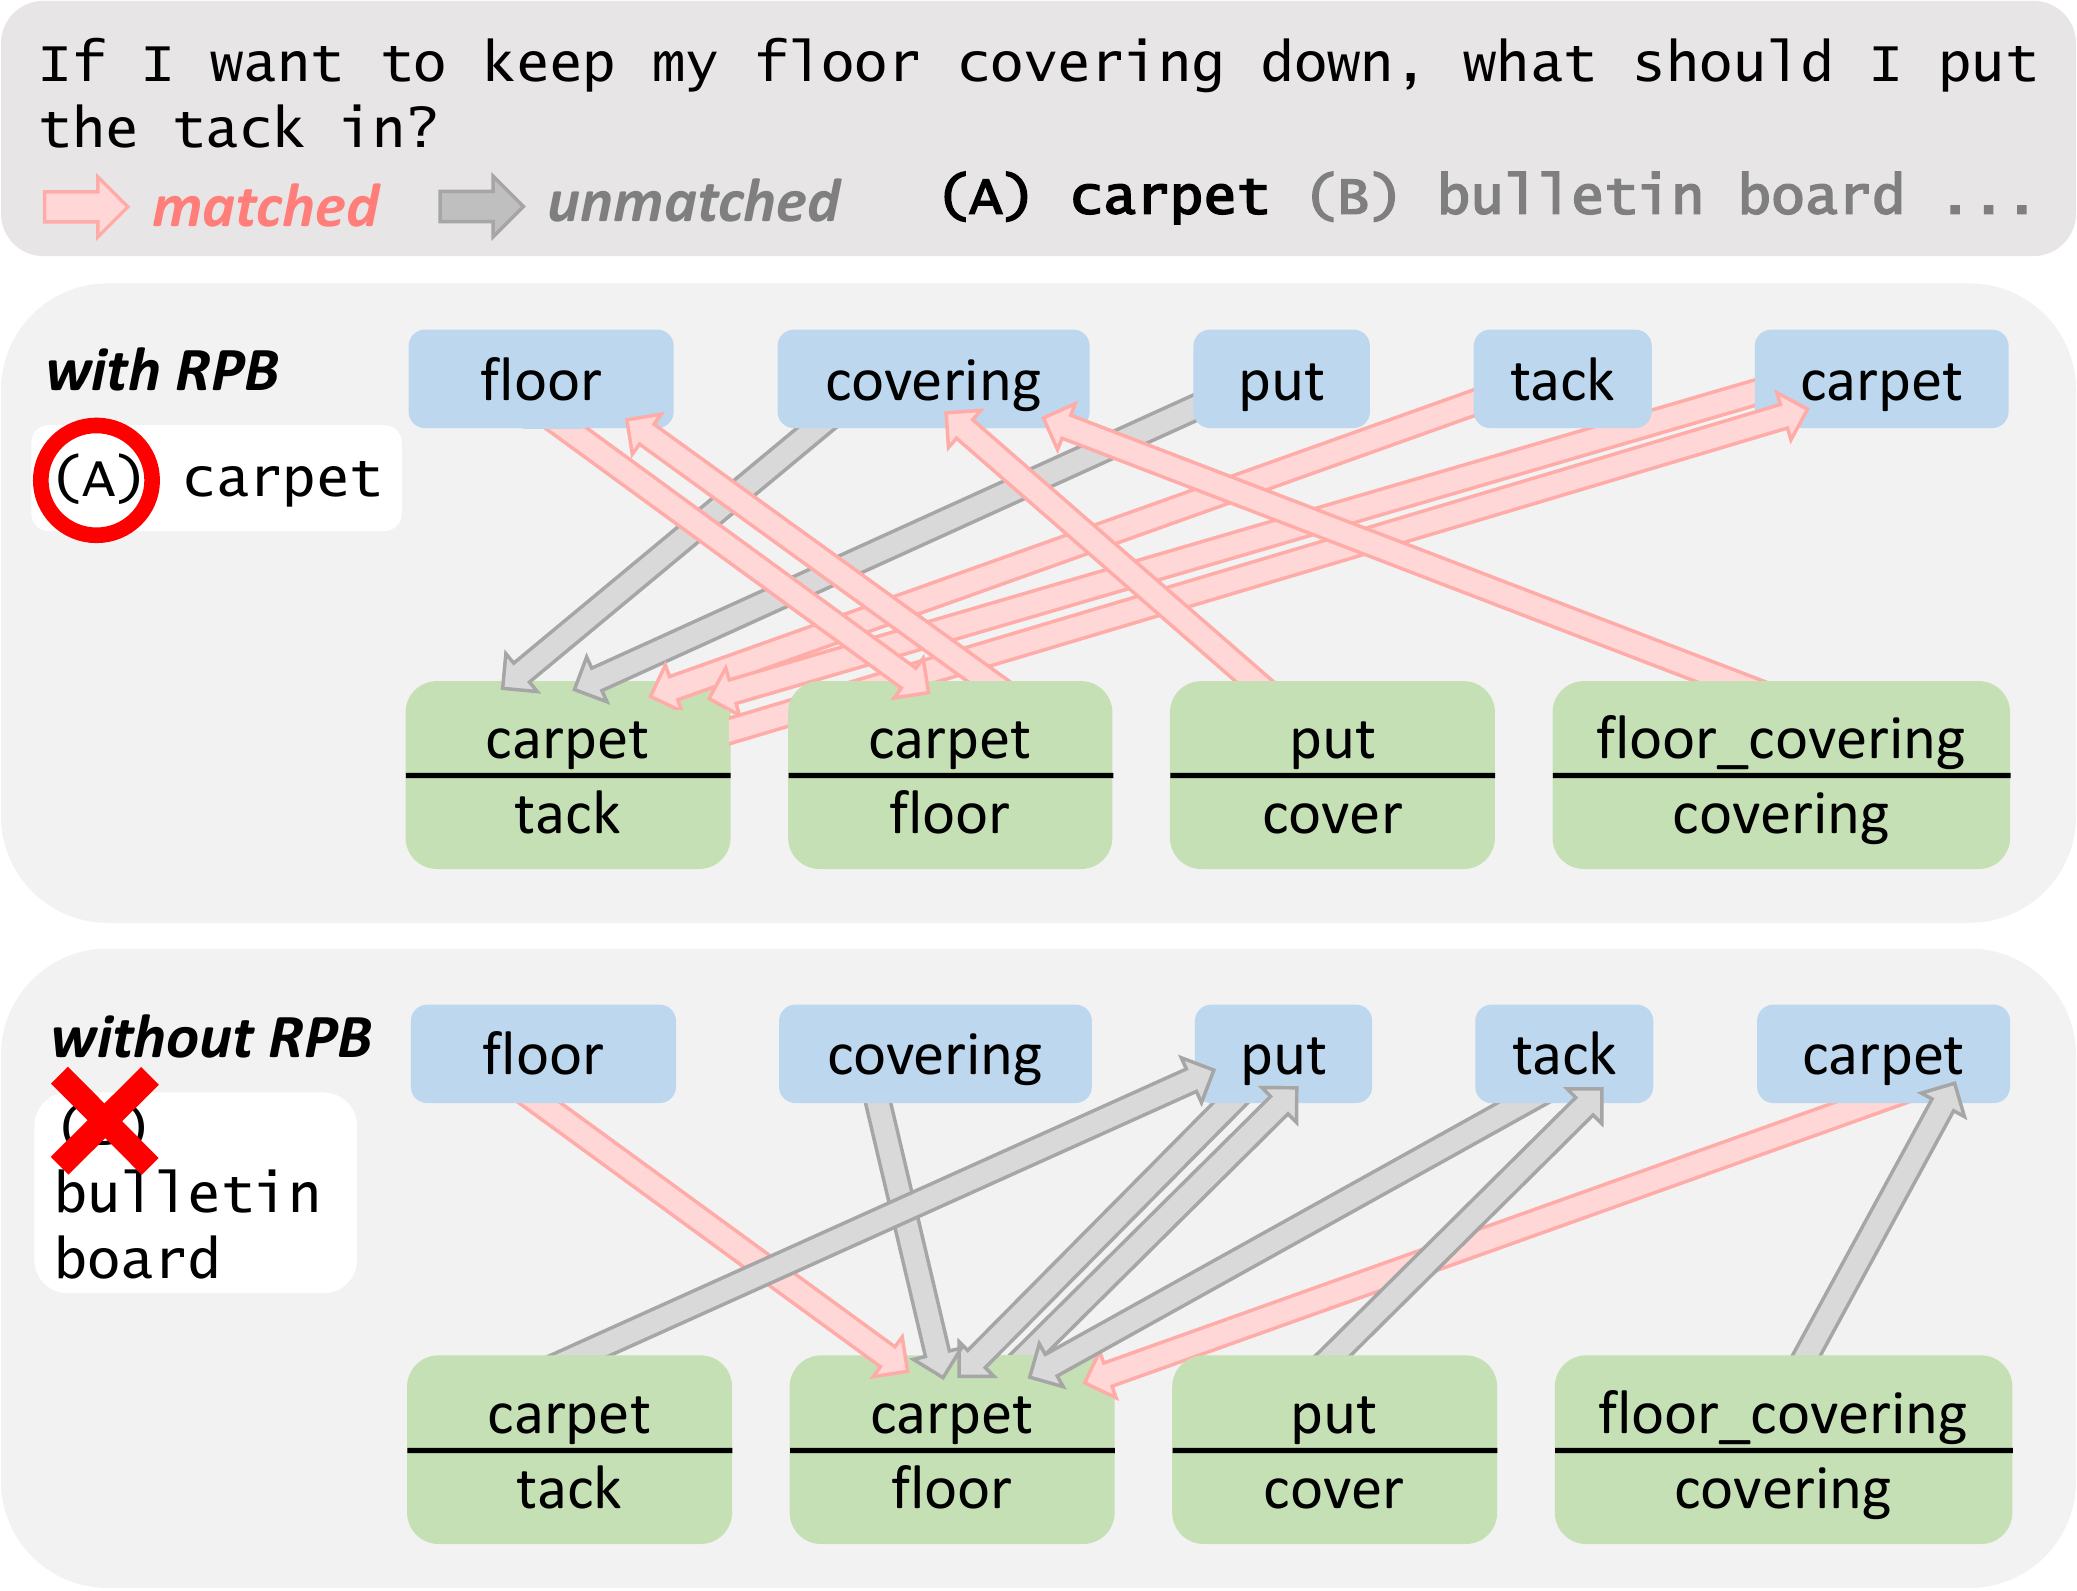}
\end{center}
% \vspace{5mm}
\caption{\textbf{Additional example of the effect of Cross-Modal Relative Position Bias.}}
\label{sup_fig:quali_matching}
\end{figure}

In Figure~\ref{sup_fig:qual} and~\ref{sup_fig:quali_matching}, we provide additional qualitative examples for what we have shown in Figure 3 and 4 of the main paper.
Similar to the main paper, the RASA maps for the correct answer choice generally show smooth values across KG and LM, whereas wrong choices tend to have weaker cross-modal attention.
Furthermore, it is also noteworthy that the Meta-Path token set size (\ie, the KG portion) is very diversified in most examples, indicating a greater KG expressivity for self-attention.
