# Supplementary material for: Relation-Aware Language-Graph Transformer for Question Answering
Source: arXiv:2212.00975 source file (2023-04-25)
Supplement: Supplementary file 3 [file suppl_choice.tex]

\begin{figure*}[t!]
\centering
% \subfigure[]{
% \includegraphics[width=1\columnwidth]{Figures/img/suppl_choice_1.pdf}
% }
\subfigure[]{
\includegraphics[width=1\columnwidth]{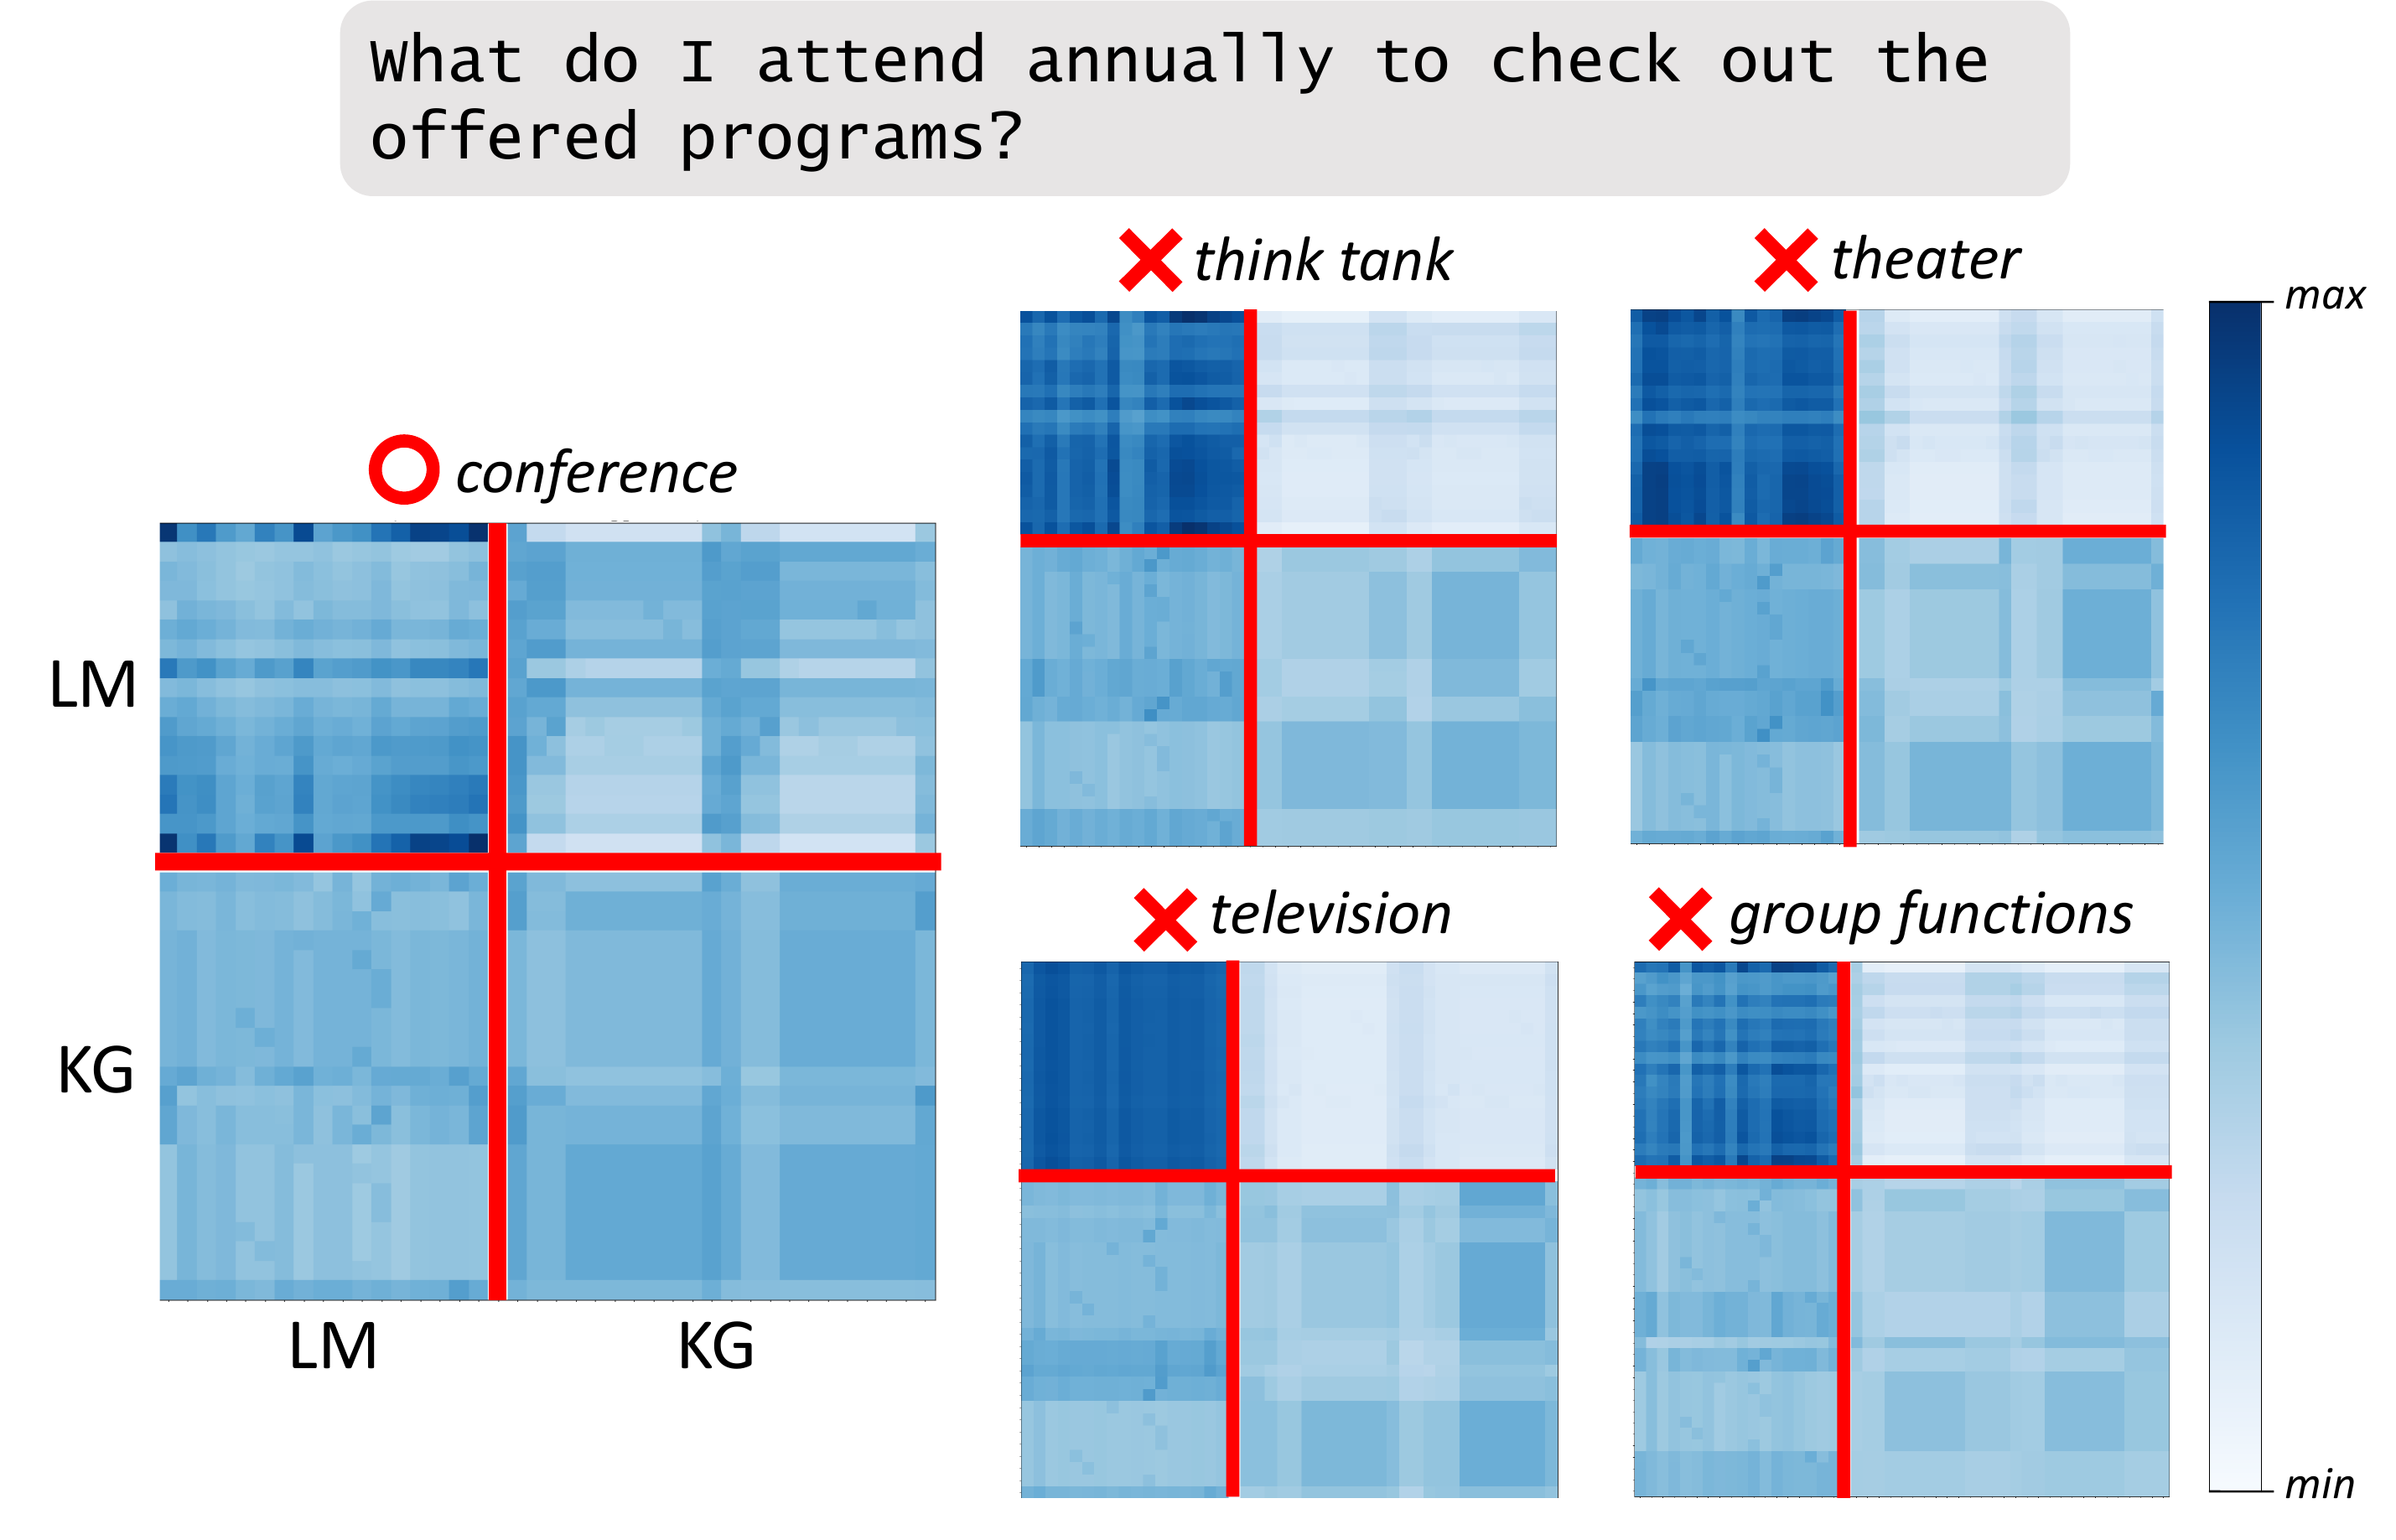}
}
\subfigure[]{
\includegraphics[width=1\columnwidth]{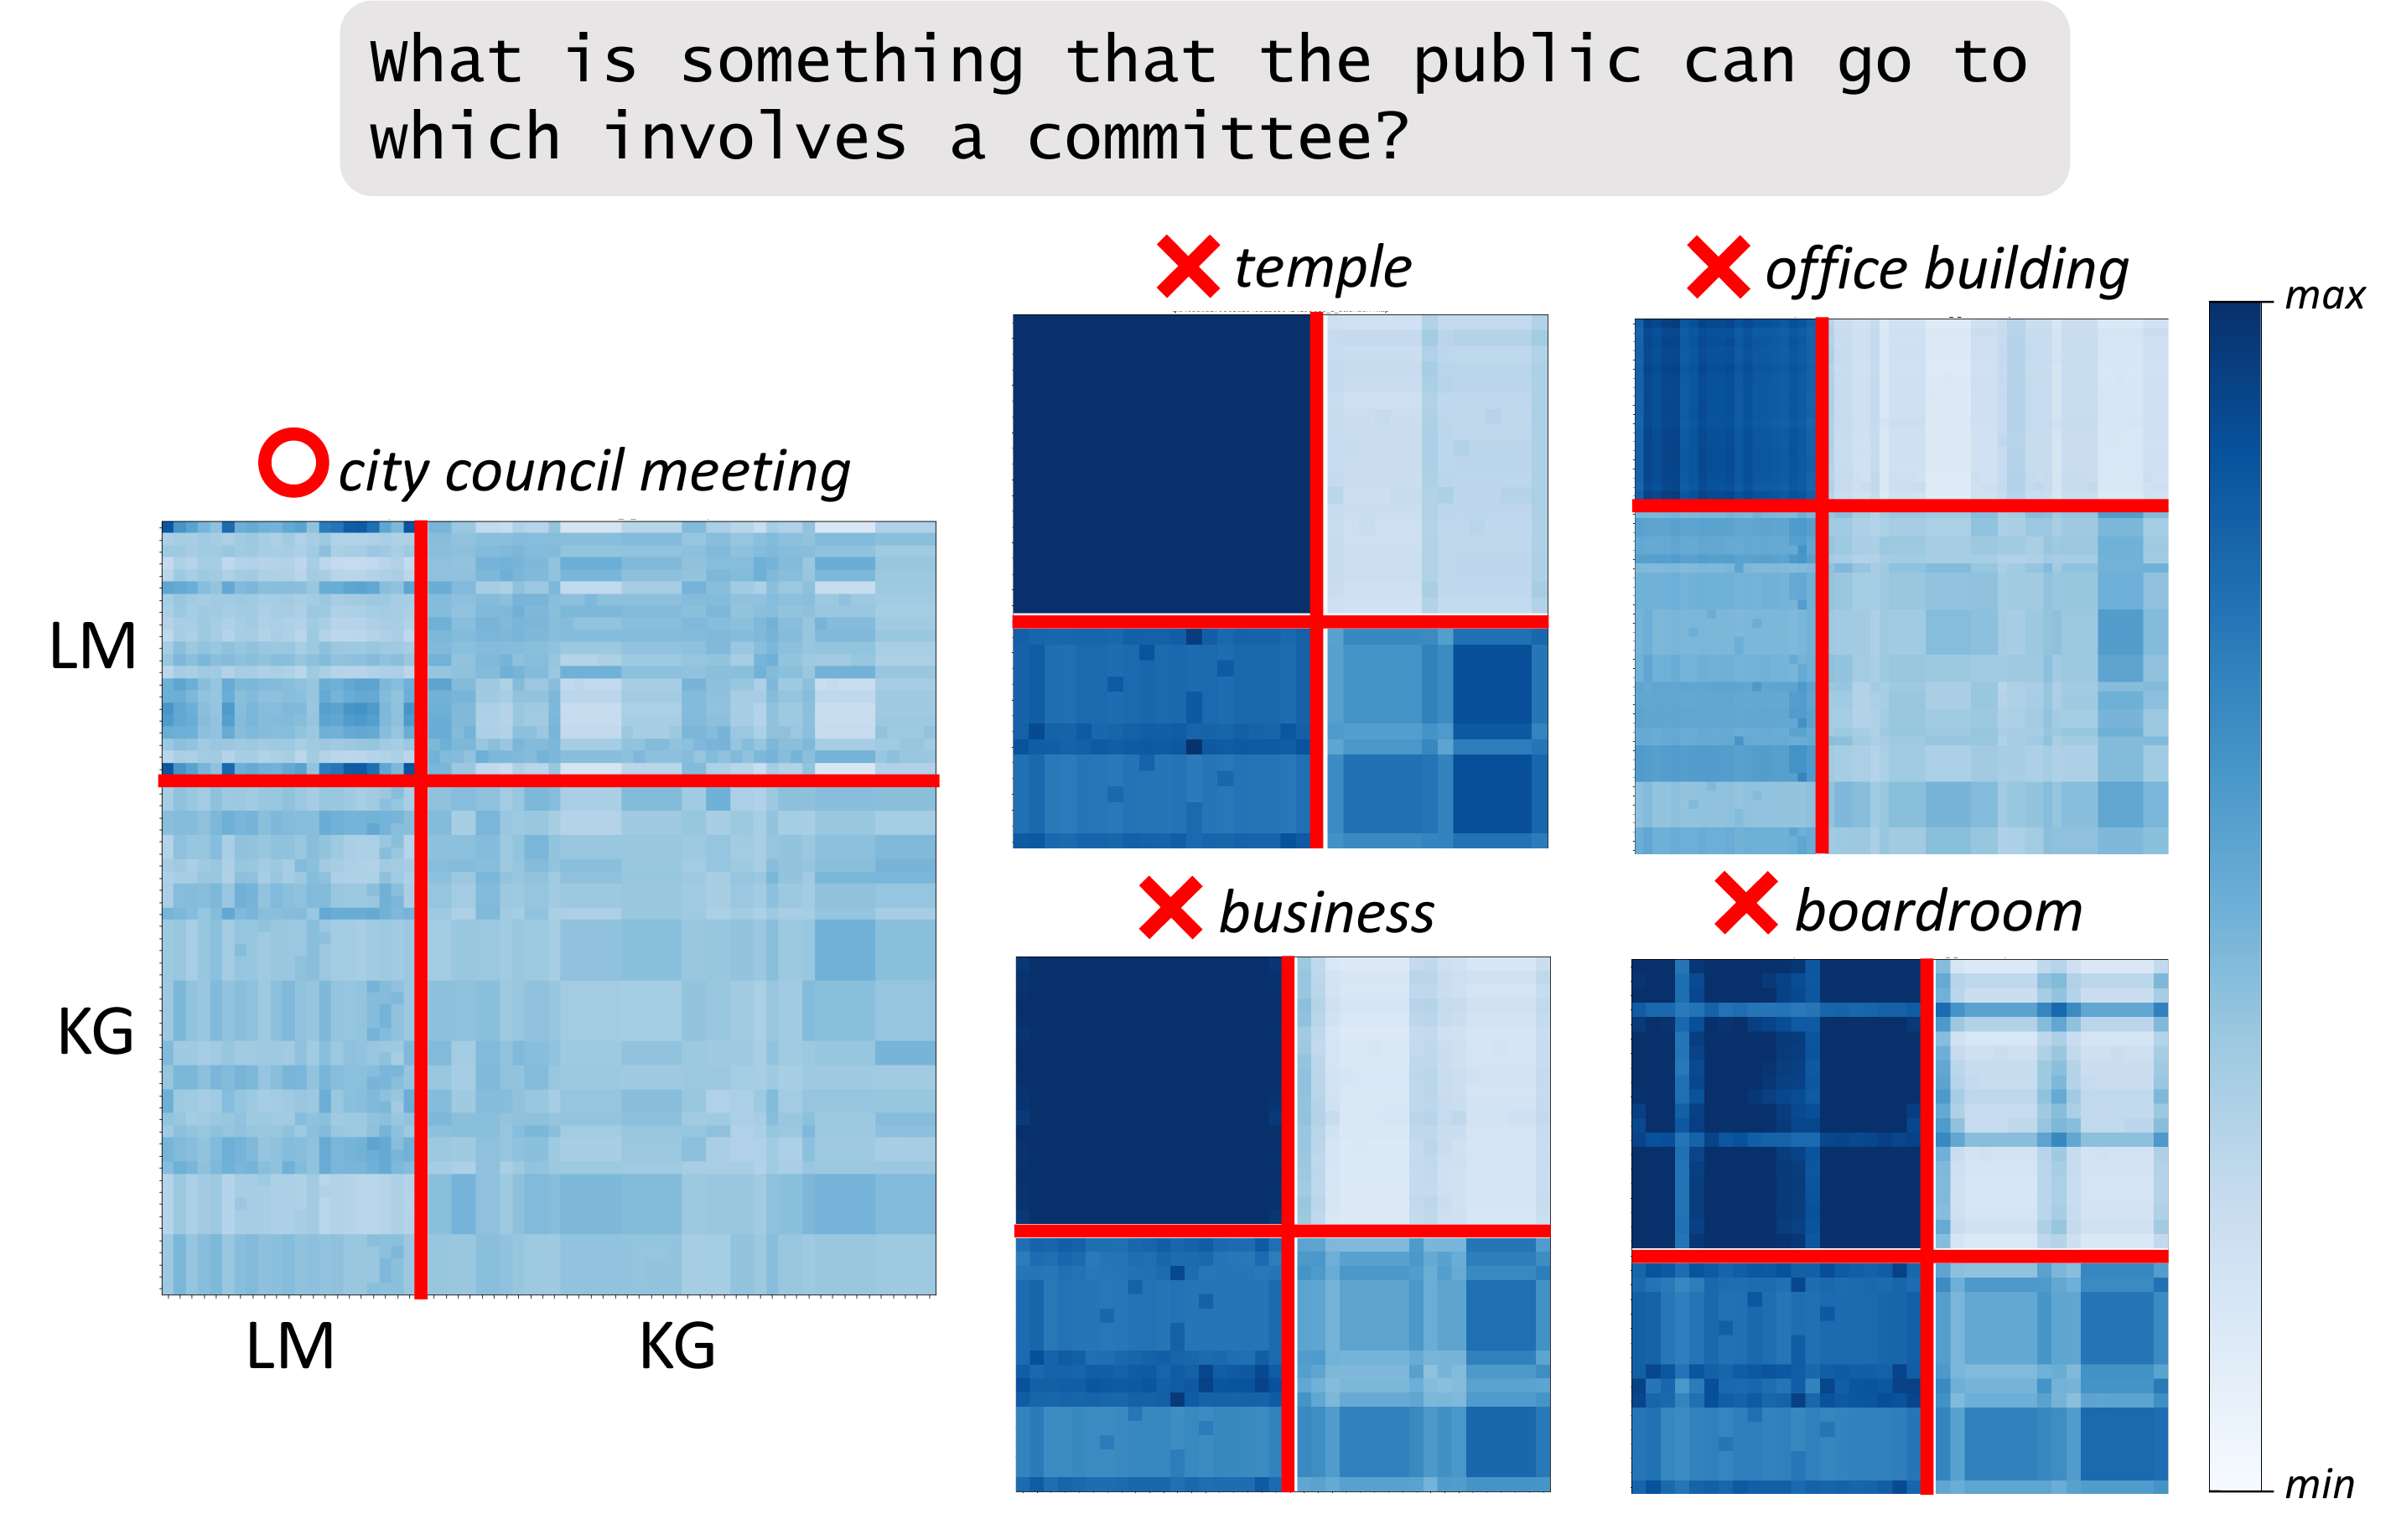}
}
% \subfigure[]{
% \includegraphics[width=1\columnwidth]{Figures/img/suppl_choice_4.pdf}
% }
\caption{ \textbf{Additional examples of QAT attention maps by each answer choice.}}
\label{sup_fig:qual}
\end{figure*}
