# Supplementary material for: Relation-Aware Language-Graph Transformer for Question Answering
Source: arXiv:2212.00975 source file (2023-04-25)
Supplement: Supplementary file 4 [file suppl_matching.tex]

\begin{figure}[t!]
\begin{center}
\includegraphics[width=1\columnwidth]{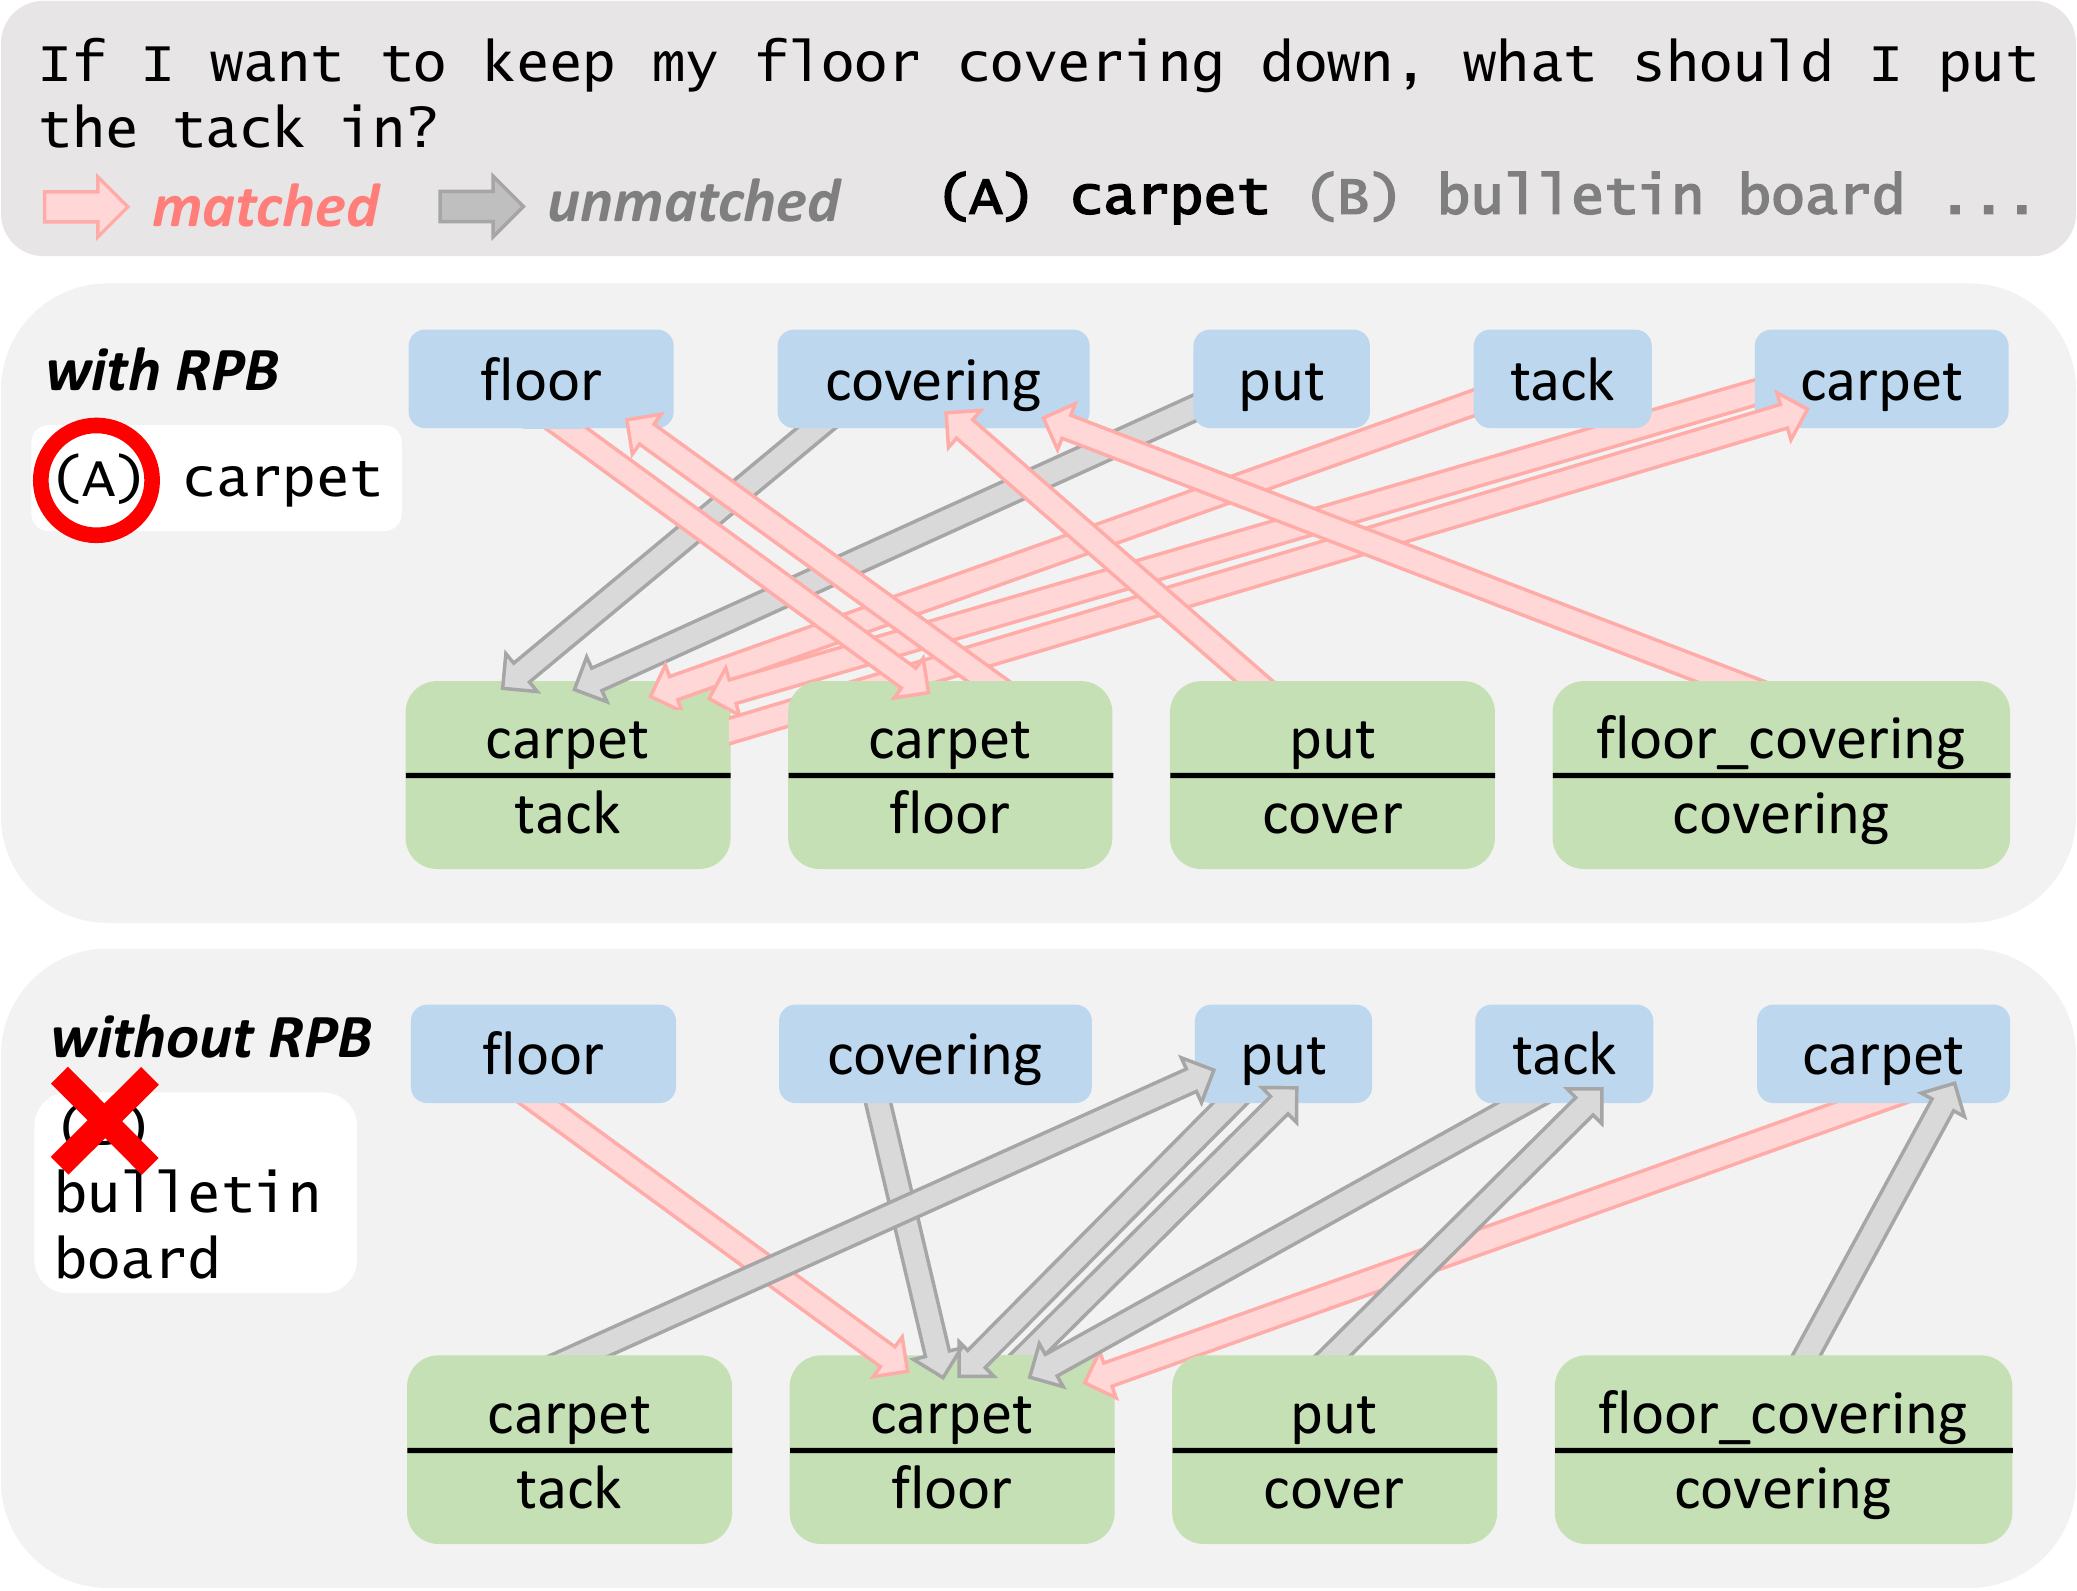}
\end{center}
% \vspace{5mm}
\caption{\textbf{Additional example of the effect of Cross-Modal Relative Position Bias.}}
\label{sup_fig:quali_matching}
\end{figure}
