# Supplementary material for: Relation-Aware Language-Graph Transformer for Question Answering
Source: arXiv:2212.00975 source file (2023-04-25)
Supplement: Supplementary file 5 [file suppl_mptoken.tex]

\begin{table}[t!]
    \centering
    \setlength{\tabcolsep}{3.5pt}
    \resizebox{0.9\columnwidth}{!}{
    \begin{tabular}{c c c}
        \toprule
        \textbf{max $K$-hops }  & \textbf{IHdev-Acc}(\%) & \textbf{IHtest-Acc}(\%) \\
        \midrule
        \midrule
        1     &      &       \\
        2     & 79.5 (± 0.4)     &  75.4 (± 0.3)     \\
        3     &      &       \\
        \bottomrule
    \end{tabular}
    }
    \caption{\textbf{Sensitivity analysis of the maximum hop used for Meta-Path tokens.}}
    \label{tab:mptoken}
\end{table}
